# Supplementary material for: DGNet: Dynamic Gradient-Guided Network for Water-Related Optics Image Enhancement
Source: arXiv:2312.06999 source file (2024-02-08)
Supplement: Supplementary file 1 [file X_suppl.tex]

\clearpage
\setcounter{page}{1}
\maketitlesupplementary

\section{Extended experiment}
\label{sec:extend}
In this section, we incorporate a substantial number of experiments to further validate the robustness of our method.

\subsection{Training advantages}
To evaluate the impact of $L_{d}^{\tau}$ in training, as shown in Fig. \ref{Fig:train_curve}, we compare the training curves with and without $L_{d}^{\tau}$ added to the total loss function. We use the MSE score curve to demonstrate the pixel-level loss during the training phase ($MSE=MAE^2$), as well as the PSNR score curve as a reference quantitative assessment metric of the network fit.
\begin{figure}[!h]
\centering 
\includegraphics[width=\linewidth]{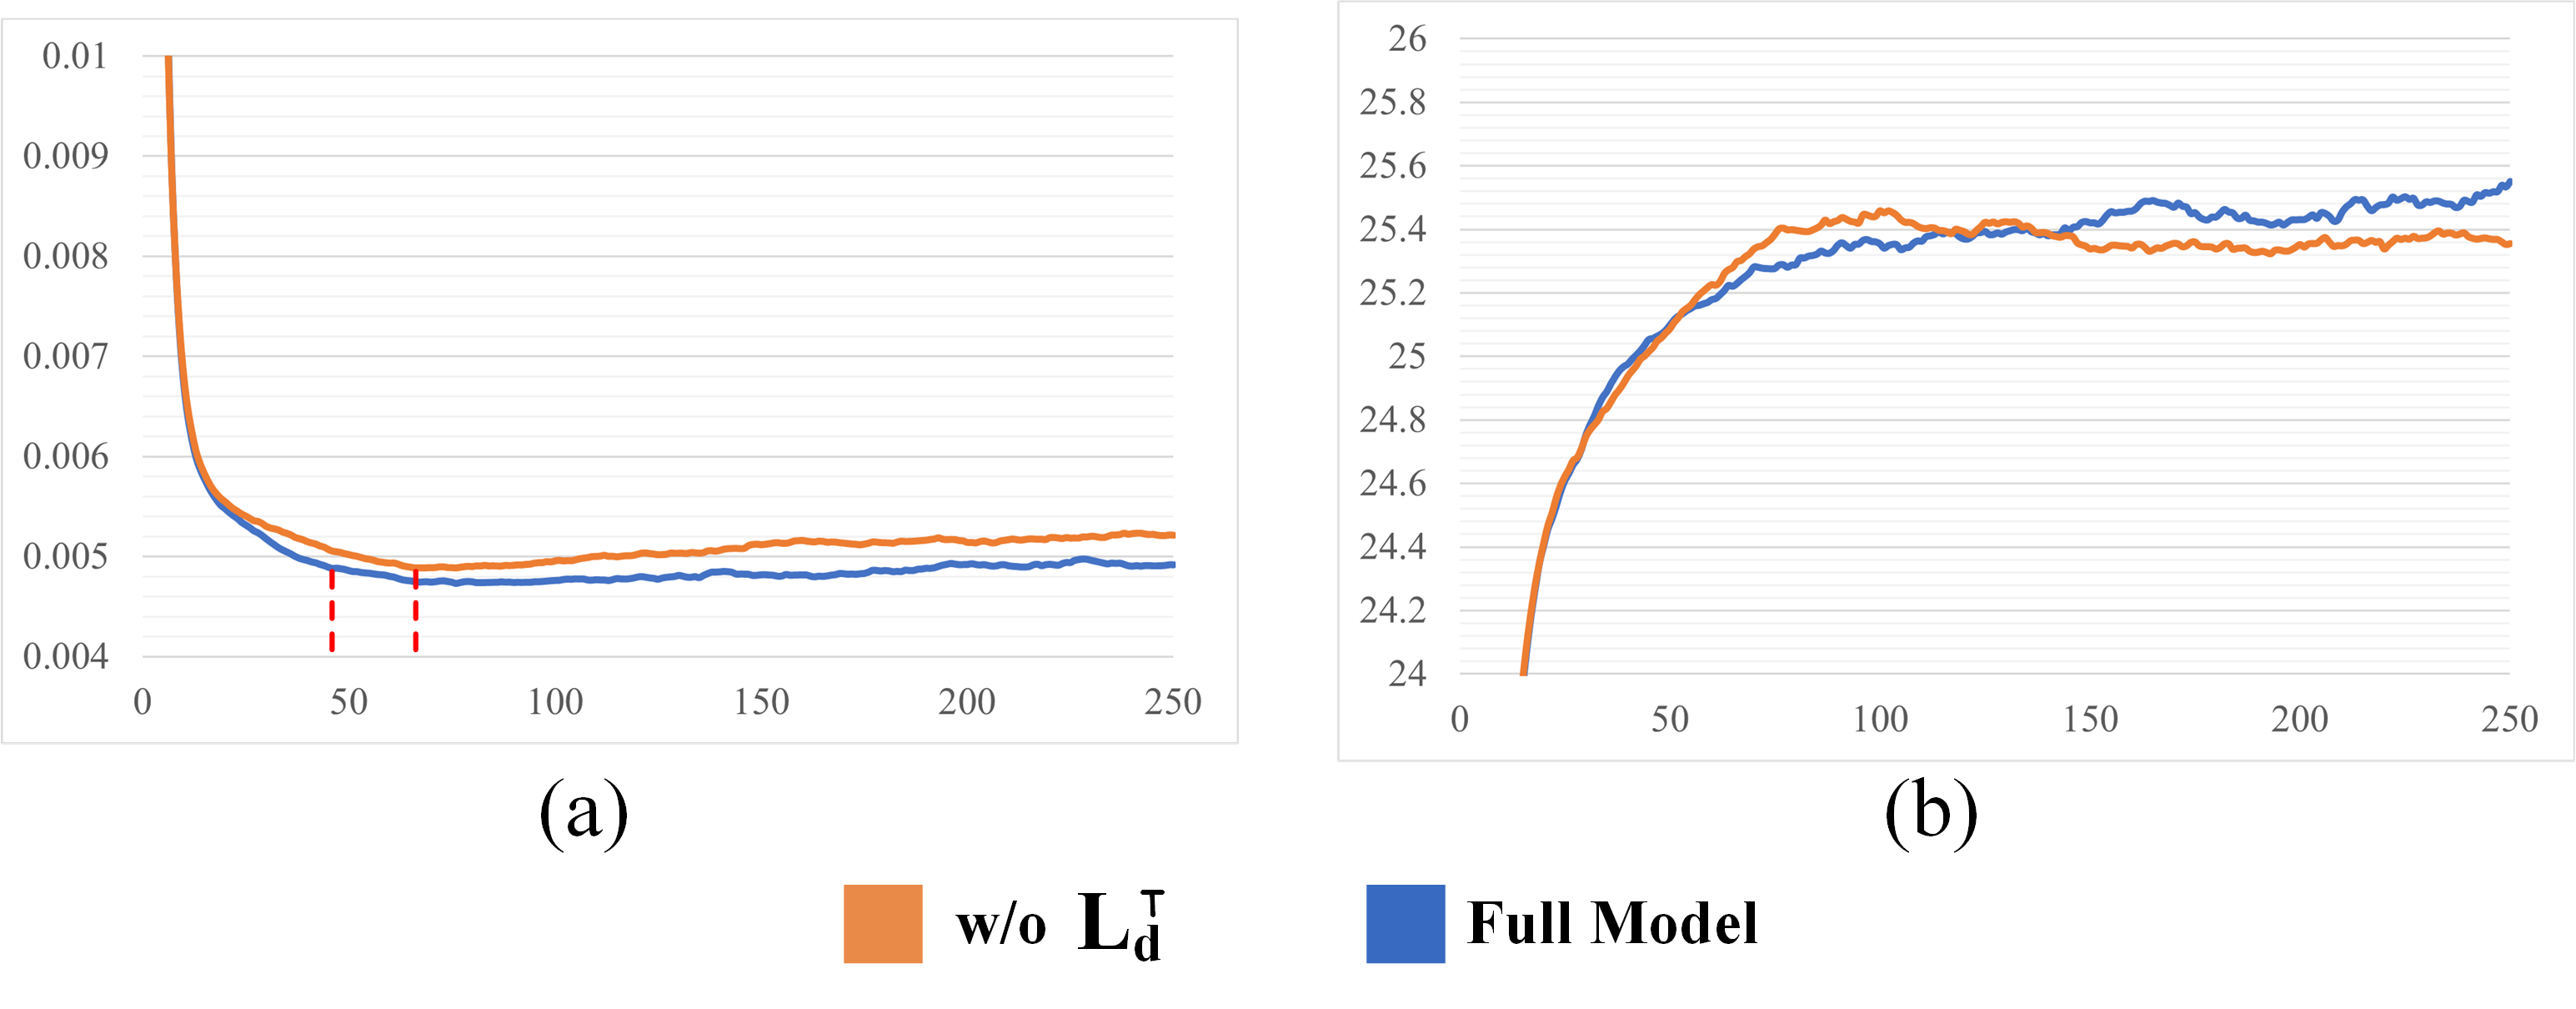}
\caption{Training curves: (a) MSE scores (lower is better); (b) PSNR scores (higher is better).}
\label{Fig:train_curve}
\end{figure}

The results show that the MSE is significantly lower with the addition of $L_{d}^{\tau}$ relative to the case without $L_{d}^{\tau}$. The network reaches the optimal level without $L_{d}^{\tau}$ in about 2/3 of the rounds, suggesting that $L_{d}^{\tau}$ has some effect of accelerating network training. Meanwhile, observing the PSNR scores as a quantitative indicator, the network with $L_{d}^{\tau}$ shows a continuous upward trend, while the network without $L_{d}^{\tau}$ shows a decline after 100 rounds, which may be caught in the local optimal solution.

The experimental results indicate that our $L_{d}^{\tau}$ effectively accelerates network training. In cases where the network gets trapped in local optima, its dynamic feature aids in rapidly escaping saddle points to seek better outcomes.

\subsection{Point Match Test}
To verify that the enhanced results of our method are beneficial for subsequent object detection tasks, we conducted keypoint detection \cite{R57PointMatch} experiments. We selected scenes with severe blue-green color bias, as shown in Fig. \ref{Fig06} (a) and (b). The enhancement results show improvements of 14.4\% and 43\%, respectively, and we also enhanced key features of both the foreground and background. This proves that our method can maintain stylistic consistency, enhance human visual perception, and improve the effectiveness of machine vision perception.

\begin{figure}[!h]
\centering 
\includegraphics[width=0.45\textwidth]{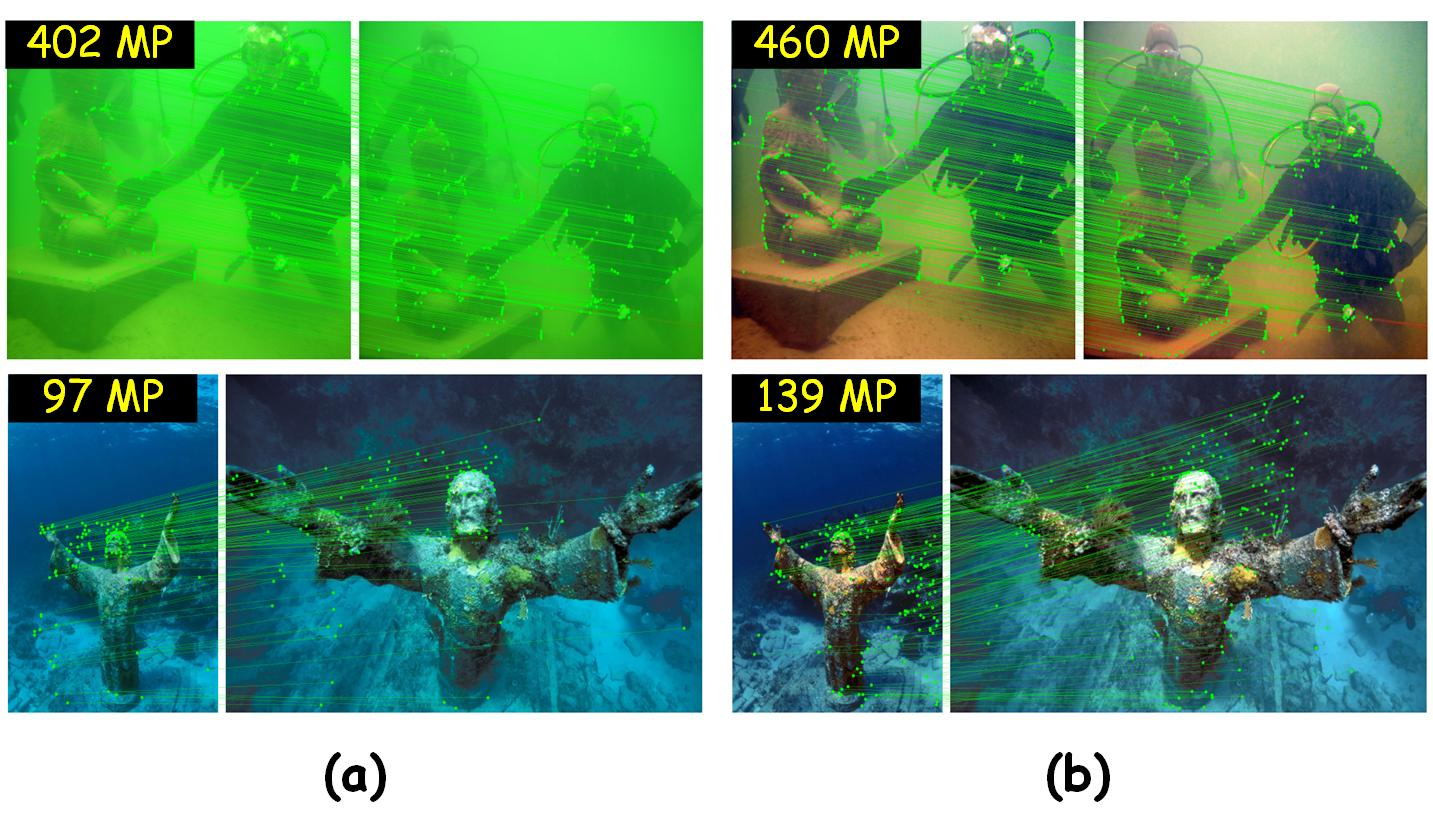}
\caption{Point match comparison in severely greenish (Top) and bluish (Bottom) Scenes: (a) raw images and (b) enhancement results. MP stands for match points. Demonstrating enhanced match counts across various angles with our method.}
\label{Fig06}
\end{figure}

\subsection{Comparison of Stylistic Consistency}
Stylistic consistency is crucial for underwater exploration. Therefore, we selected different viewpoint images from the LLFF dataset \cite{R56llff} as the test set and compared them with three advanced methods: NAFNet (ECCV’22) \cite{R36NAFNet}, Restormer (CVPR’22) \cite{R35Restormer}, and Semi-UIR (CVPR’23) \cite{R37SemiUIR}. The enhancement effects are illustrated in Fig. \ref{Fig09:std}.
\begin{figure*}[!th]
\centering 
\includegraphics[width=0.95\textwidth]{sec/Fig09_std.jpg}
\caption{Visual presentation on the LLFF dataset \cite{R56llff}. where the images are presented for different viewpoints in the same scene and can therefore be used to assess stylistic consistency. The scores in the upper right corner of the image are as in Eq. \ref{eq:std}, with yellow being the optimal score (lower is better).}
\label{Fig09:std}
\end{figure*}

Based on the gray world assumption, the goal of image restoration is to make the color distribution uniform throughout the image, i.e., the average color should be gray. We designed to use the standard deviation of the channel mean for quantitatively evaluating the white balance effect of the image, and this metric can be expressed as follows:
\begin{align}
score = \sqrt{\frac{1}{3} \sum_{i}^{\hat{r}, \hat{g}, \hat{b}} (i - \hat{I})^2}
\label{eq:std}
\end{align}
where $\hat{r}, \hat{g}, \hat{b}$ represent the mean value of the rgb channel and $\hat{I}$ represents the mean value of all pixels. This score is displayed in the upper right corner of the image.

Our method achieves the best results in different angle images of the same scene, and the difference between the maximum and minimum scores is only 1.26, compared to 1.98 for the original image, 4.09 for Restormer \cite{R35Restormer}, 2.98 for NAF \cite{R36NAFNet}, and 4.24 for Semi-UIR \cite{R37SemiUIR}.The differences are larger than that of the original image except for our method, which indicates that our method excels in image restoration style consistency.

\section{Visual Results and Failure Cases}
\subsection{More Visual Result}
As demonstrated by several experiments, our method achieves strikingly excellent results, with the quality of the recovered images even surpassing the Ground-True (GT) image of the UIEB dataset \cite{R18WaterNet} in some of them, as shown in Fig. \ref{Fig:res_val}. This shows that our approach addresses the issue of poor quality in some GT image.

\subsection{Failure Cases}
Our approach significantly reduces the amount of parameters and computational resources required, but it also has some limitations. We hope that future work can further enhance this. Unconventional image scenes (e.g., using special scenes or customized lenses) may adversely affect the recovery performance of our method, as shown in Fig. \ref{Fig:lim}. This may be caused by the fact that the network is trained only on the UIEB dataset \cite{R18WaterNet}, which does not have unconventional data to cope with special scenes.
\begin{figure}[!h]
\centering 
\includegraphics[width=0.35\textwidth]{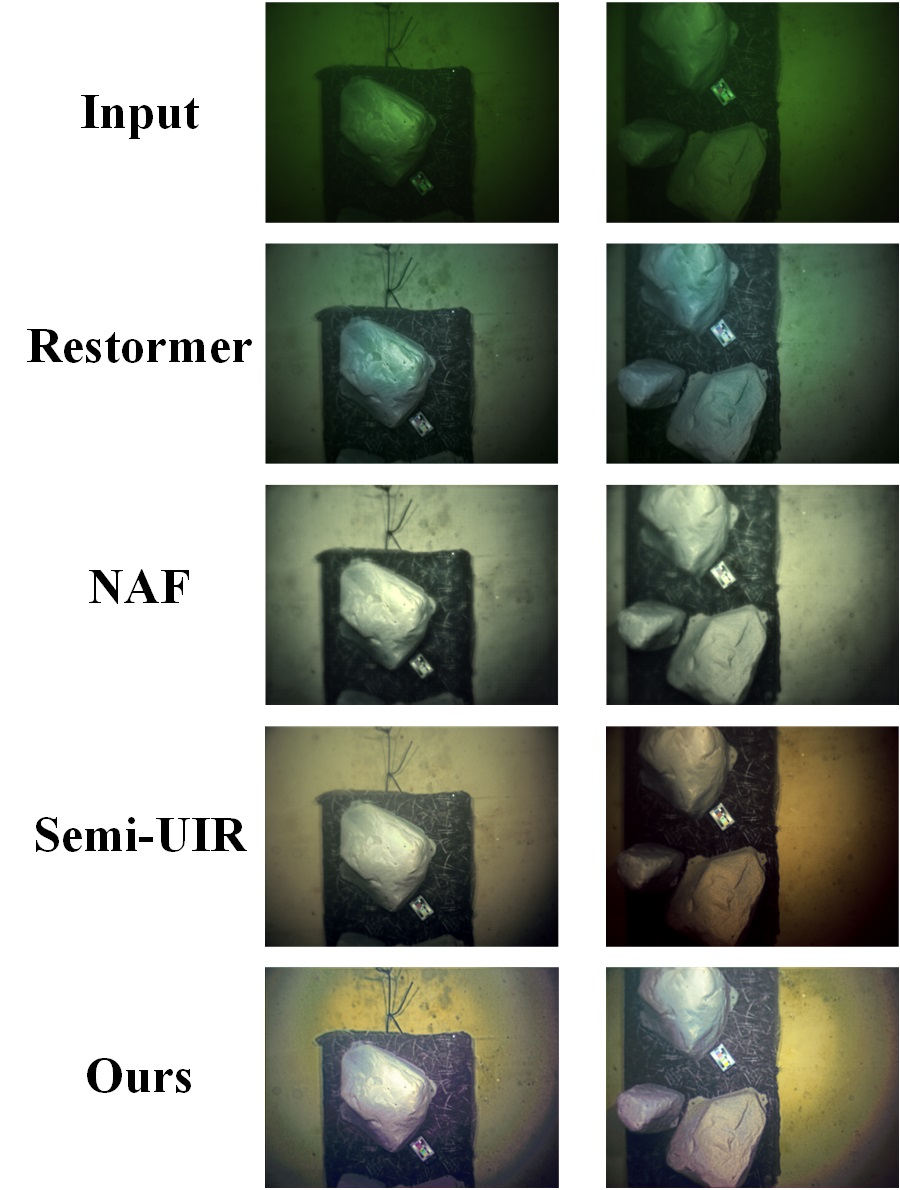}
\caption{Error Enhancement for Exception Scenarios. The images are selected from the UWbundle dataset \cite{R55Limit}.}
\label{Fig:lim}
\end{figure}

The recovery results of the two sample images show that none of the other methods remove the color deviation, and although our method effectively removes the color deviation, there is a certain deviation in the pixel recovery. As the pixels get farther and farther away from the center point of the camera, the deviation will get bigger and bigger. In future work, we will solve this problem from the perspective of data enhancement.

\begin{figure*}[!h]
\centering 
\includegraphics[width=0.5\textwidth]{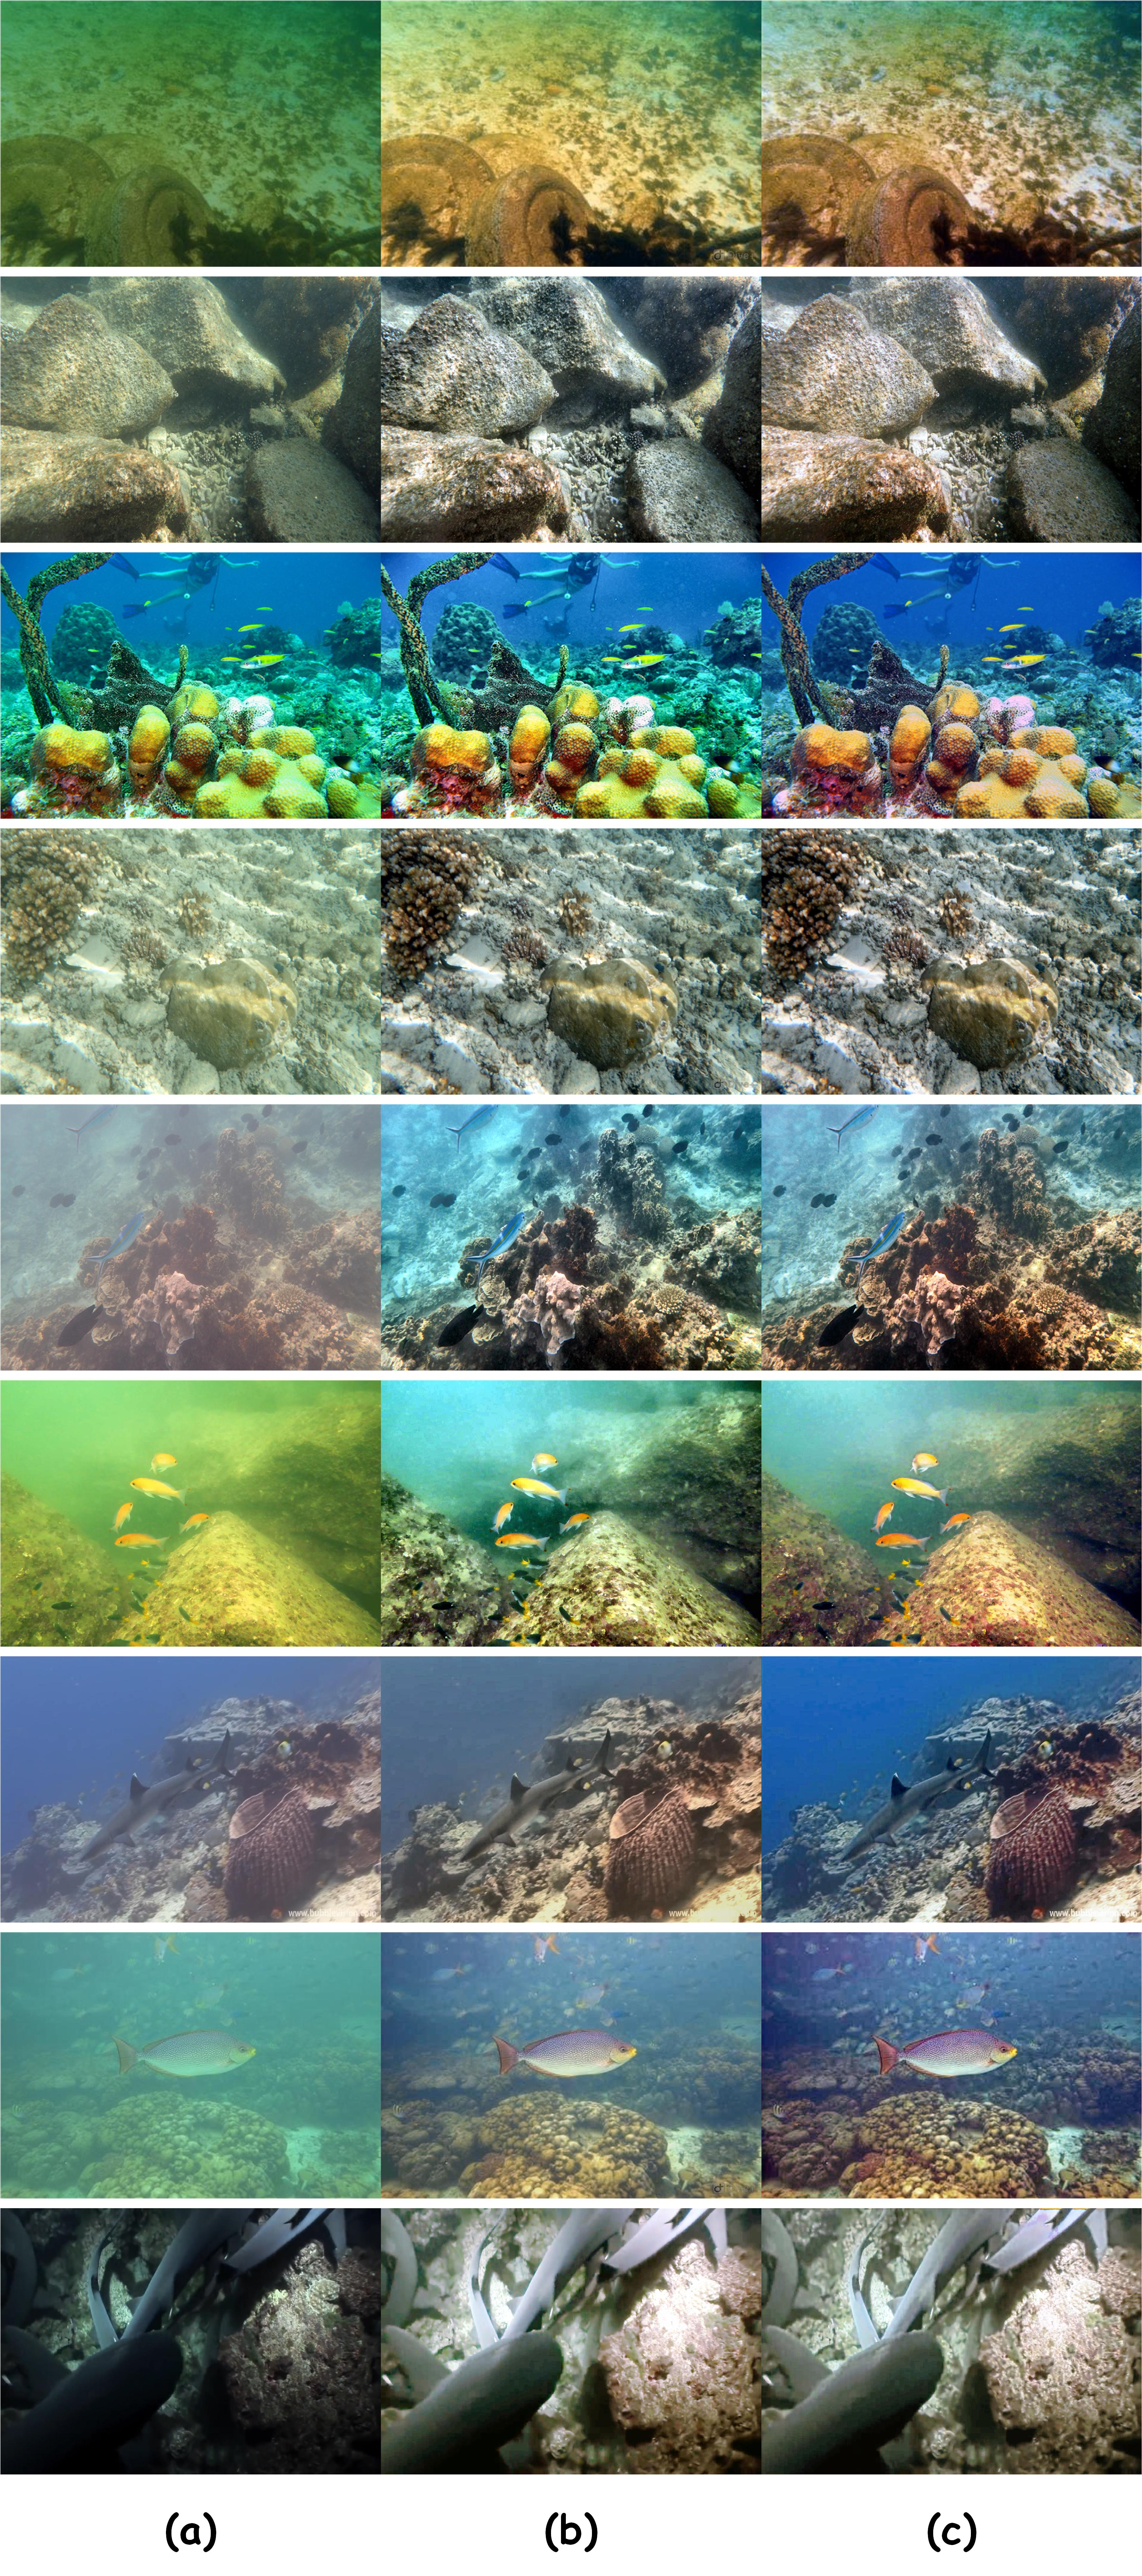}
\caption{Visual comparison on UIEB V90 \cite{R18WaterNet}. (a) original image,  (b) Ground Truth, and (c) enhanced results by our method.}
\label{Fig:res_val}
\end{figure*}
